# Supplementary material for: Dynamical solid-liquid transition through oscillatory shear
Source: arXiv:1809.08874 ancillary file (2018-09-24)
Supplement: Supplementary file 1 [file sm-oscillatoryshear.pdf]

# Electronic Supplementary Information

# Dynamical solid-liquid phase transition through oscillatory shear

Éric Brillaux[1, 2] and Francesco Turci[2, *]
[1] *École Normale Supérieure de Lyon, 65 Allée d'Italie, 69007 Lyon, France*
[2] *H.H. Wills Physics Laboratory, Tyndall Avenue, Bristol, United Kingdom*

## I. VINET'S EQUATION OF STATE FOR THE 3D BINARY LJ SYSTEM

In order to prepare the system at zero pressure we determine the equation of state of the two-component solid. The equation of state assumed for the crystal is inferred following Vinet *et al.* [1]. This approach neglects the binary nature of the material and considers the average potential energy $U$ in relation to the average particle-particle distance $r$.

In general, the pressure at constant number of particles and temperature is related to the free energy $F$ and the volume $V$ by

$$p = -\left(\frac{\partial F}{\partial V}\right)_{T,N} \approx -\left(\frac{\partial U}{\partial V}\right)_{T} \tag{S1}$$

where the approximation is valid if the entropic contributions to the free energy are weakly dependent on the volume.

Since the volume $V$ is proportional to $r^3$ and given that the Lennard-Jones potential energy is $U \propto (\sigma_{eff}/r)^{12} - (\sigma_{eff}/r)^6$, $\sigma_{eff}$ being the effective (as we disregard the distinction between A and B particles) potential range, then it is possible to relate the pressure to $r$:

$$p = -\left(\frac{\partial V}{\partial r}\right)_{T}^{-1}\left(\frac{\partial U}{\partial r}\right)_{T} \tag{S2}$$

$$\propto r^{-2}\left[2\left(\frac{\sigma_{eff}}{r}\right)^{13} - \left(\frac{\sigma_{eff}}{r}\right)^{7}\right] \tag{S3}$$

$$\propto 2\left(\frac{\sigma_{eff}}{r}\right)^{15} - \left(\frac{\sigma_{eff}}{r}\right)^{9} \tag{S4}$$

The above expression can be cast into a more condensed form if the pressure is expressed in terms of the parameter $x = \rho/\rho_0 \propto r^{-3}$, where $\rho_0$ is the density at zero pressure and $B_0 = \rho(\partial p/\partial \rho)_T(p = 0)$ is the bulk modulus at zero pressure:

$$p = 2B_0\, x^3(x^2 - 1) \tag{S5}$$

Fitting the the simulations with this expression, see Fig. S1(a), we can also extract the bulk modulus $B_0$ and the density at zero pressure as in Fig. S1(b).

## II. FINITE-SIZE EFFECTS ON RELAXATION TIMES AND CRITICAL STRAIN AMPLITUDE IN THE 3D BINARY LJ SYSTEM

For the three-dimensional LJ binary crystal we have considered systems of sizes $N = 768, 1500, 12000, 96000, 768000$, looking for eventual signatures of strong finite size effects. Not without surprise, we have found that the amorphization transition is very similar for very different system sizes.

For example, in Fig. S2(a) we show the relaxation times as a function of the strain amplitude $\gamma_0$ for the considered system sizes at temperature $T = 0.336$. Not only the qualitative behaviour (i.e., a divergence of the relaxation time) is

* Author to whom correspondence should be addressed. Electronic mail:f.turci@bristol.ac.uk

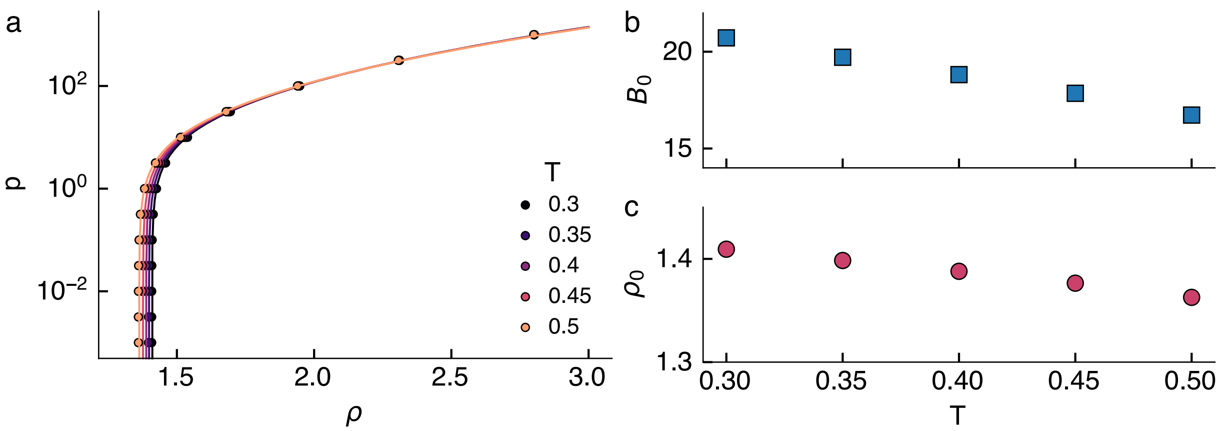


FIG. S1. **Equation of state of the binary Lennard-Jones crystal.** (a) Molecular dynamics results for pressure as a function of the density at several temperatures (symbols) fitted by Vinet's approximation (continuous lines), Eq. S5, where $x = \rho/\rho_0$. The temperature-dependent fitting parameters are (b) the bulk modulus $B_0$ and (c) the zero-pressure density $\rho_0$.

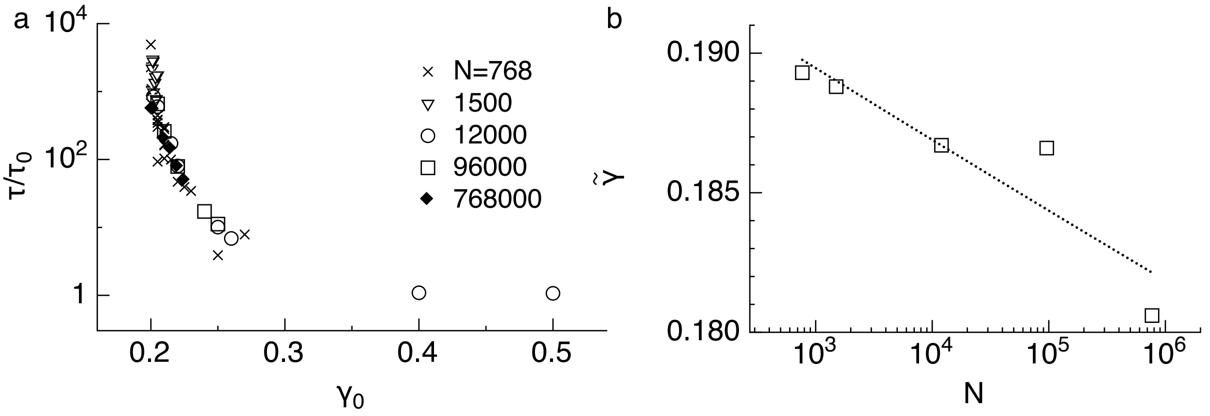


FIG. S2. **Finite-size effects on the amorphization of the 3d binary LJ crystal.** (a) Relaxation time to the amorphous state as a function of the strain amplitude at $T = 0.336$. (b) Estimates of the critical strain amplitude as a function of the system size. The dotted line is a power law fit $\gamma_c \sim N^{-0.006}$.

the same for the several systems under study, but the quantitative value of the relaxation times are in good agreement between systems of size 768 particles and system $10^3$ times larger.

However, a weak, systematic finite-size effect can be measured from the estimates of the critical strain $\tilde{\gamma}$ at which the relaxation times appear to diverge. To compute $\tilde{\gamma}$ we proceed as follows: we assume the scaling law $\tau \sim (\gamma - \tilde{\gamma})^{-\nu}$ with $\nu = 3$ (see main text) and we find the value of $\tilde{\gamma}$ that optimizes the $R^2$ value of the linear regression between $\log \tau$ and $\log(\gamma - \tilde{\gamma})$. In Fig. S2(b) we show that the critical strain $\tilde{\gamma}$ varies modestly ($\approx 5\%$) when the system sizes increases by a factor $10^3$. In particular, the critical value *decreases* as the system size is increased, showing that smaller systems can sustain slightly larger strain amplitudes. Stronger correlations induced by the periodic boundary conditions on smaller systems are possible sources of such an effect.

## III. RESIDUAL ORIENTATIONAL ORDER IN THE 3D BINARY LJ AMORPHOUS STATE

The amorphous state obtained from the three-dimensional LJ binary crystal is such that the original $Al_2Cu$ periodicity is broken. However, some remnants of the crystalline order can still be identified in the final disordered steady state. This is the case, for instance, of partial orientational order of the small (B) particles that form the spindle of bicapped antiprisms.

To this purpose, we define a suitable orientational order parameter measuring the global alignment of the spindles. For every antiprism, the unitary orientation vector $\boldsymbol{w}$ of the $A_8B_3$ clusters (and only them) is determined by the mean direction pointed by the three internal B particles. By convention the vector is always set with a positive $z$

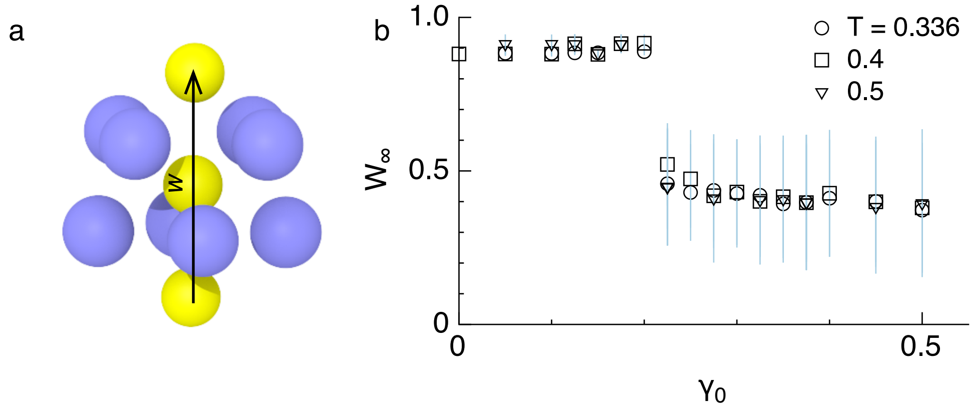


FIG. S3. **Residual spindle orientation.** (a) Bicapped square antiprism, composed of a spindle of three small B particles (yellow) and eight large A particles. The arrow represents the orientation vector $\boldsymbol{w}$. (b) Global orientation parameter $W_\infty$ for a system of $N = 1200$ particles of temperature $T - 0.336, 0.4, 0.5$ as a function fo the strain amplitude $\gamma_0$. Errorbars correspond to a standard deviation.

component. The global orientation vector $\boldsymbol{w}$ is then computed for each time $t$ according to Eq. S6.

$$\langle \boldsymbol{w} \rangle = \frac{1}{N_{\text{antiprisms}}} \sum_{i=1}^{N_c} \boldsymbol{w_i} \tag{S6}$$

where $N_{\text{antiprisms}}$ is the total number of antiprisms. Were the system totally isotropic, $\langle \boldsymbol{w} \rangle$ would take the following value:

$$\langle \boldsymbol{n} \rangle = \frac{1}{2\pi} \int_0^{2\pi} \mathrm{d}\phi \int_0^{\pi/2} \mathrm{d}\theta \cos\theta \sin\theta \, \boldsymbol{e_z} = \frac{1}{4} \left[\cos(2\theta)\right]_{\pi/2}^{0} \boldsymbol{e_z} = \frac{1}{2} \boldsymbol{e_z} \tag{S7}$$

where $\phi$ and $\theta$ are the angular spherical coordinates. Likewise, in a perfectly ordered crystal where all clusters are aligned in the $z$ direction, $\langle \boldsymbol{w} \rangle$ would be equal to $\boldsymbol{e_z}$. Taking this into account, we define $W$ as

$$W = 2 \left| \langle \boldsymbol{w} \rangle \right| - 1, \tag{S8}$$

such that it is zero for an isotropic material and one for a perfectly aligned system, regardless of the orientation which is known to be always close to $\boldsymbol{e_z}$. In particular we take the long time value $W_\infty$ to quantify the degree of residual orientational alignment at steady state.

In Fig. S3 we show that the orientation of the spindles changes discontinuously as the strain amplitude is increased. In particular, while for small $\gamma_0$ the reversible oscillatory crystalline state has $W_\infty$ close to unity, in the amorphous state this is much lower ($W_\infty(\gamma_0 > \tilde{\gamma}) \approx 0.3$) but significantly larger than zero, indicating that parts of the system retain partial memory of the original crystalline state even after hundreds of cycles in the amorphous steady state.

## IV. SUPPLEMENTARY VIDEOS

- **sv1-LJ2d.mp4** The video shows the complete oscillations of the 2D Lennard-Jones system at temperature $T = 0.4$ and strain amplitude $\gamma_0 = 0.205$ color-coded by the modulus of the orientational order parameter.

- **sv2-LJ3dfccbcc.mp4** The video shows the time-evolution of the 3D Lennard-Jones crystal at temperature $T = 0.6$ and strain amplitude $\gamma_0 = 0.28$. In particular, it shows the initial amorphization of the fcc order, and the subsequent nucleation of the bcc order. We employ VoroTop [2] as implemented in Ovito [3] to identify fcc (blue), hcp (green), mixed fcc/hcp (light green), bcc (orange) and icosahedral (yellow) environments. Snapshots are taken only after entire oscillations, hence the box is always orthorombic.

- **sv3-768Kparticles.mp4** The video shows the order-disorder transition in a large 3D binary Lennard-Jones system of 768000 particles at temperature $T = 0.336$ and strain amplitude $\gamma_0 = 0.215$. Large and small particles

are in red and blue respectively, while in green we represent the interface between ordered and amorphous regions (grey facets are in the periodic dimension). Snapshots are taken only after entire oscillations, hence the box is always orthorombic.

- **sv4-nucleus2.5.mp4** The video shows the growth of a seeded amorphous nucleus of radius $R = 2.5\sigma_A$ in the 3D binary Lennard-Jones crystal at $T = 0.336$ and $\gamma_0 = 0.21$. Large and small particles are in red and blue respectively, while in green we represent the interface between ordered and amorphous regions. Snapshots are taken only after entire oscillations, hence the box is always orthorombic.

[1] P. Vinet, J. R. Smith, J. Ferrante, and J. H. Rose, Physical Review B **35**, 1945 (1987).
[2] E. A. Lazar, Modelling and Simulation in Materials Science and Engineering **26**, 015011 (2017).
[3] A. Stukowski, Modelling and Simulation in Materials Science and Engineering **18**, 015012 (2009).
